# Supplementary material for: Spontaneous flows in active smectics with dislocations
Source: arXiv:2405.18250 ancillary file (2024-05-28)
Supplement: Supplementary file 1 [file SI_Lin_ActiveSmectics_28052024.pdf]

# Supplemental Material
# Spontaneous flows in active smectics with dislocations

Shao-Zhen Lin,[1] Frank Jülicher,[2,3] Jacques Prost,[4,5] and Jean-François Rupprecht[1]

[1]*Aix Marseille Univ, Université de Toulon, CNRS, CPT (UMR 7332), Turing Centre for Living Systems, Marseille, France*
[2]*Max Planck Institute for the Physics of Complex Systems, 01187 Dresden, Germany*
[3]*Cluster of Excellence, Physics of Life, TU Dresden, 01307 Dresden, Germany*
[4]*Laboratoire Physico-Chimie Curie, UMR 168, Institut Curie, PSL Research University, CNRS, Sorbonne Université, 75005 Paris, France*
[5]*Mechanobiology Institute, National University of Singapore, 117411 Singapore*

(Dated: May 28, 2024)

**Contents**

**I. Theory of active smectics with dislocations** 2
A. Governing equations 2
B. Linear stability analysis 4
1. Specific role of $\tilde{\lambda}_m$: stability requirement in the passive case 7
2. Specific role of $\nu_K$: stability requirement in the passive case 7
3. General case: small-scale stability in arbitrary directions 7
4. General case: large-scale stability in arbitrary directions 8
5. General case: stability along the smectic layers direction 9
6. General case: stability along the normal to the smectic layers direction 11

**II. Theory of active smectics without dislocations** 16
A. Governing equations 16
B. Mapping to previous work on active smectics without dislocations. 16
C. Linear stability analysis 17

**References** 20

# I. THEORY OF ACTIVE SMECTICS WITH DISLOCATIONS

## A. Governing equations

We briefly recall the set of governing equations for active smectic layers in two-dimensional space defined in the main text.

1. The layer number conservation equation reads:

$$\frac{\partial (m\boldsymbol{k})}{\partial t} + \nabla J_m = -\hat{\boldsymbol{z}} \times \left(\boldsymbol{J}^+ - \boldsymbol{J}^-\right), \tag{S1}$$

where the layer flux

$$J_m = m\boldsymbol{v}\cdot\boldsymbol{k} - D_m\boldsymbol{k}\cdot\nabla m + \lambda_m \nabla\cdot\boldsymbol{k} + \xi_m\nabla^2(\nabla\cdot\boldsymbol{k}) + d\boldsymbol{k}\cdot\nabla\left(n^+ + n^-\right), \tag{S2}$$

and the dislocation flux

$$\boldsymbol{J}^{\pm} = n^{\pm}\boldsymbol{v} - D_n\nabla n^{\pm} \pm \nu n^{\pm}\left(m - m_H\right)\boldsymbol{k}\times\hat{\boldsymbol{z}} \pm \nu_K n^{\pm}\left(\nabla\left(\nabla\cdot\boldsymbol{k}\right)\times\hat{\boldsymbol{z}}\right). \tag{S3}$$

Note that, in the main text, we have ignored the last term $d\boldsymbol{k}\cdot\nabla\left(n^+ + n^-\right)$ in $J_m$ (Eq. (S2)); in Sec. I B, we show that such a term does not affect the linear stability of active smectic layers. Thus, we set it to be zero ($d = 0$) in our present study.

2. The dynamic evolution of the number density of dislocations reads:

$$\frac{\partial n^{\pm}}{\partial t} + \nabla\cdot\boldsymbol{J}^{\pm} = -\alpha n^+ n^- + \beta. \tag{S4}$$

3. The topological constraint on layers entails that:

$$\nabla\times(m\boldsymbol{k}) = \left(n^+ - n^-\right)\hat{\boldsymbol{z}}. \tag{S5}$$

4. The force balance equation is:

$$\nabla\cdot\boldsymbol{\sigma} - \lambda\boldsymbol{v} + \boldsymbol{T} = \boldsymbol{0}, \tag{S6}$$

where the stress reads

$$\boldsymbol{\sigma} = -P\boldsymbol{I} + 2\eta\boldsymbol{E} - B\frac{m - m_S}{m_H}\left(\boldsymbol{k}\otimes\boldsymbol{k} - \frac{1}{2}\boldsymbol{I}\right) + K\left[\boldsymbol{k}\otimes\nabla\left(\nabla\cdot\boldsymbol{k}\right) + \nabla\left(\nabla\cdot\boldsymbol{k}\right)\otimes\boldsymbol{k} - \boldsymbol{k}\cdot\nabla\left(\nabla\cdot\boldsymbol{k}\right)\boldsymbol{I}\right], \tag{S7}$$

and the active traction $\boldsymbol{T}$ reads:

$$\boldsymbol{T} = -\zeta_s\left(\nabla\cdot\boldsymbol{k}\right)\boldsymbol{k} - \zeta_b\boldsymbol{k}\cdot\nabla\boldsymbol{k} - \chi\nabla m - \mu_d(n^+ - n^-)\left(m - m_H\right)\boldsymbol{k}\times\hat{\boldsymbol{z}}, \tag{S8}$$

including:

(a) the active traction forces induced by the splay (the $\zeta_s$ term) and bend deformations (the $\zeta_b$ term) of smectic components,

(b) the layer spacing inhomogeneity $\chi\nabla m$, which does not affect the dynamics of the active smectic layers but just renormalizes the hydrodynamic pressure, i.e., $P \to P + \chi m$. We refer to this term as active pressure and, in our present study, set it to zero ($\chi = 0$).

(c) a specific contribution of dislocations, $\mu_d$; this term does not affect the linear stability of active smectic layers; thus, in our present study, we consider $\mu_d = 0$.

5. The incompressibility equation imposes that:

$$\nabla\cdot\boldsymbol{v} = 0. \tag{S9}$$

We point out that the set of generic equations remains unchanged under the mirror symmetry operation $\boldsymbol{k} \leftrightarrow -\boldsymbol{k}$.

*Proof of the consistency of Eqs.* (S1) *and* (S4) *with Eq.* (S5). – Applying the differential operator $\nabla\times$ to Eq. (S1), we obtain:

$$\frac{\partial[\nabla \times (m\boldsymbol{k})]}{\partial t} = -(\nabla \cdot \boldsymbol{J}^+ - \nabla \cdot \boldsymbol{J}^-)\hat{\boldsymbol{z}}, \tag{S10}$$

where we have used the identity $\nabla \times (\boldsymbol{A} \times \boldsymbol{B}) = (\nabla \cdot \boldsymbol{B})\boldsymbol{A} - (\nabla \cdot \boldsymbol{A})\boldsymbol{B} + (\boldsymbol{B} \cdot \nabla)\boldsymbol{A} - (\boldsymbol{A} \cdot \nabla)\boldsymbol{B}$. The dynamic evolution of the number density of dislocations leads to:

$$\frac{\partial(n^+ - n^-)}{\partial t} + (\nabla \cdot \boldsymbol{J}^+ - \nabla \cdot \boldsymbol{J}^-) = 0. \tag{S11}$$

Thus, combining Eq. (S10) and Eq. (S11), we obtain:

$$\frac{\partial[\nabla \times (m\boldsymbol{k}) - (n^+ - n^-)\hat{\boldsymbol{z}}]}{\partial t} = 0. \tag{S12}$$

This equation always holds due to the topological constraint Eq. (S5).

*Detailed expressions of the governing equations.*– Substituting Eqs. (S2) and (S3) to Eqs. (S1) and (S4), we obtain,

$$\begin{aligned}\frac{\partial \boldsymbol{M}}{\partial t} =& -\nabla\left(\boldsymbol{v}\cdot\boldsymbol{M}\right) + D_m \nabla\boldsymbol{k}\cdot\nabla m + D_m \boldsymbol{k}\cdot\nabla\nabla m - \lambda_m \nabla\left(\nabla\cdot\boldsymbol{k}\right) - \xi_m \nabla\nabla^2\left(\nabla\cdot\boldsymbol{k}\right) - d\nabla\boldsymbol{k}\cdot\nabla n - d\boldsymbol{k}\cdot\left(\nabla\nabla n\right)\\ & - w\hat{\boldsymbol{z}}\times\boldsymbol{v} + D_n \hat{\boldsymbol{z}}\times\nabla w - \nu n\left(m - m_H\right)\boldsymbol{k} - \nu_K n \nabla\left(\nabla\cdot\boldsymbol{k}\right),\end{aligned} \tag{S13}$$

and

$$\begin{aligned}\frac{\partial n}{\partial t} =& -\nabla n\cdot\boldsymbol{v} + D_n \nabla^2 n - \nu\left[\left(m - m_H\right)\left(\nabla w\times\boldsymbol{k}\right) + w\left(\nabla m\times\boldsymbol{k}\right) + w\left(m - m_H\right)\left(\nabla\times\boldsymbol{k}\right)\right]\cdot\hat{\boldsymbol{z}}\\ & - \nu_K\left[\nabla w\times\nabla(\nabla\cdot\boldsymbol{k})\right]\cdot\hat{\boldsymbol{z}} - \frac{1}{2}\alpha\left(n^2 - w^2\right) + 2\beta,\end{aligned} \tag{S14}$$

where $\boldsymbol{M} = m\boldsymbol{k}$ is the smectic director field; $n = n^+ + n^-$ is the total number density of $\pm1$ dislocations; $w = n^+ - n^- = (\nabla \times \boldsymbol{M}) \cdot \hat{\boldsymbol{z}} = \partial M_y/\partial x - \partial M_x/\partial y$ is the difference of the number density of $\pm1$ dislocations.

Next, we will give detailed expressions of the governing equations. The smectic director field $\boldsymbol{M} = M_x\hat{\boldsymbol{x}} + M_y\hat{\boldsymbol{y}}$ evolves as:

$$\begin{aligned}\frac{\partial M_x}{\partial t} =& -\left(M_x\frac{\partial v_x}{\partial x} + M_y\frac{\partial v_y}{\partial x} + v_x\frac{\partial M_x}{\partial x} + v_y\frac{\partial M_x}{\partial y}\right) + D_m\left(k_x\frac{\partial^2 m}{\partial x^2} + k_y\frac{\partial^2 m}{\partial x\partial y} + \frac{\partial k_x}{\partial x}\frac{\partial m}{\partial x} + \frac{\partial k_y}{\partial x}\frac{\partial m}{\partial y}\right)\\ & - \lambda_m\left(\frac{\partial^2 k_x}{\partial x^2} + \frac{\partial^2 k_y}{\partial x\partial y}\right) - \xi_m\left(\frac{\partial^4 k_x}{\partial x^4} + \frac{\partial^4 k_x}{\partial x^2\partial y^2} + \frac{\partial^4 k_y}{\partial x^3\partial y} + \frac{\partial^4 k_y}{\partial x\partial y^3}\right) + D_n\left(\frac{\partial^2 M_x}{\partial y^2} - \frac{\partial^2 M_y}{\partial x\partial y}\right)\\ & - d\left(k_x\frac{\partial^2 n}{\partial x^2} + k_y\frac{\partial^2 n}{\partial x\partial y} + \frac{\partial k_x}{\partial x}\frac{\partial n}{\partial x} + \frac{\partial k_y}{\partial x}\frac{\partial n}{\partial y}\right) - \nu n\left(m - m_H\right)k_x - \nu_K n\left(\frac{\partial^2 k_x}{\partial x^2} + \frac{\partial^2 k_y}{\partial x\partial y}\right),\end{aligned} \tag{S15}$$

$$\begin{aligned}\frac{\partial M_y}{\partial t} =& -\left(M_x\frac{\partial v_x}{\partial y} + M_y\frac{\partial v_y}{\partial y} + v_x\frac{\partial M_y}{\partial x} + v_y\frac{\partial M_y}{\partial y}\right) + D_m\left(k_x\frac{\partial^2 m}{\partial x\partial y} + k_y\frac{\partial^2 m}{\partial y^2} + \frac{\partial k_x}{\partial y}\frac{\partial m}{\partial x} + \frac{\partial k_y}{\partial y}\frac{\partial m}{\partial y}\right)\\ & - \lambda_m\left(\frac{\partial^2 k_x}{\partial x\partial y} + \frac{\partial^2 k_y}{\partial y^2}\right) - \xi_m\left(\frac{\partial^4 k_x}{\partial x^3\partial y} + \frac{\partial^4 k_x}{\partial x\partial y^3} + \frac{\partial^4 k_y}{\partial x^2\partial y^2} + \frac{\partial^4 k_y}{\partial y^4}\right) + D_n\left(\frac{\partial^2 M_y}{\partial x^2} - \frac{\partial^2 M_x}{\partial x\partial y}\right)\\ & - d\left(k_x\frac{\partial^2 n}{\partial x\partial y} + k_y\frac{\partial^2 n}{\partial y^2} + \frac{\partial k_x}{\partial y}\frac{\partial n}{\partial x} + \frac{\partial k_y}{\partial y}\frac{\partial n}{\partial y}\right) - \nu n\left(m - m_H\right)k_y - \nu_K n\left(\frac{\partial^2 k_x}{\partial x\partial y} + \frac{\partial^2 k_y}{\partial y^2}\right).\end{aligned} \tag{S16}$$

The total number density of positive and negative dislocations $n$ evolves as:

$$\begin{aligned}\frac{\partial n}{\partial t} =& -\left(v_x\frac{\partial n}{\partial x} + v_y\frac{\partial n}{\partial y}\right) + D_n\left(\frac{\partial^2 n}{\partial x^2} + \frac{\partial^2 n}{\partial y^2}\right) - \nu\left(m - m_H\right)\left[k_y\left(\frac{\partial^2 M_y}{\partial x^2} - \frac{\partial^2 M_x}{\partial x\partial y}\right) - k_x\left(\frac{\partial^2 M_y}{\partial x\partial y} - \frac{\partial^2 M_x}{\partial y^2}\right)\right]\\ & - \nu_K\left[\left(\frac{\partial^2 k_x}{\partial x\partial y} + \frac{\partial^2 k_y}{\partial y^2}\right)\left(\frac{\partial^2 M_y}{\partial x^2} - \frac{\partial^2 M_x}{\partial x\partial y}\right) + \left(\frac{\partial^2 k_x}{\partial x^2} + \frac{\partial^2 k_y}{\partial x\partial y}\right)\left(\frac{\partial^2 M_x}{\partial y^2} - \frac{\partial^2 M_y}{\partial x\partial y}\right)\right]\\ & - \nu w\left[k_y\frac{\partial m}{\partial x} - k_x\frac{\partial m}{\partial y} + \left(m - m_H\right)\left(\frac{\partial k_y}{\partial x} - \frac{\partial k_x}{\partial y}\right)\right] - \frac{1}{2}\alpha\left(n^2 - w^2\right) + 2\beta.\end{aligned} \tag{S17}$$

The force balance equation reads:

$$-\lambda v_x + \eta\Big(\frac{\partial^2 v_x}{\partial x^2} + \frac{\partial^2 v_x}{\partial y^2}\Big) = \frac{\partial P}{\partial x} - \frac{\partial \mathrm{X}}{\partial x} - \frac{\partial \mathrm{Y}}{\partial y} - T_x, \tag{S18}$$

$$-\lambda v_y + \eta\Big(\frac{\partial^2 v_y}{\partial x^2} + \frac{\partial^2 v_y}{\partial y^2}\Big) = \frac{\partial P}{\partial y} + \frac{\partial \mathrm{X}}{\partial y} - \frac{\partial \mathrm{Y}}{\partial x} - T_y. \tag{S19}$$

where

$$\begin{aligned} \mathrm{X} &= -B\frac{m - m_S}{m_H}\Big(k_x^2 - \frac{1}{2}\Big) + K\left[k_x\left(\frac{\partial^2 k_x}{\partial x^2} + \frac{\partial^2 k_y}{\partial x \partial y}\right) - k_y\left(\frac{\partial^2 k_x}{\partial x \partial y} + \frac{\partial^2 k_y}{\partial y^2}\right)\right], \\ \mathrm{Y} &= -B\frac{m - m_S}{m_H}k_x k_y + K\left[k_x\left(\frac{\partial^2 k_x}{\partial x \partial y} + \frac{\partial^2 k_y}{\partial y^2}\right) + k_y\left(\frac{\partial^2 k_x}{\partial x^2} + \frac{\partial^2 k_y}{\partial x \partial y}\right)\right], \end{aligned} \tag{S20}$$

and

$$\begin{aligned} T_x &= -\zeta_s k_x\left(\frac{\partial k_x}{\partial x} + \frac{\partial k_y}{\partial y}\right) - \zeta_b\left(k_x\frac{\partial k_x}{\partial x} + k_y\frac{\partial k_x}{\partial y}\right) - \chi\frac{\partial m}{\partial x} - \mu_d w\,(m - m_H)\,k_y, \\ T_y &= -\zeta_s k_y\left(\frac{\partial k_x}{\partial x} + \frac{\partial k_y}{\partial y}\right) - \zeta_b\left(k_x\frac{\partial k_y}{\partial x} + k_y\frac{\partial k_y}{\partial y}\right) - \chi\frac{\partial m}{\partial y} + \mu_d w\,(m - m_H)\,k_x. \end{aligned} \tag{S21}$$

The incompressibility condition is enforced by the pressure $P$, which satisfies the following Poisson equation:

$$\frac{\partial^2 P}{\partial x^2} + \frac{\partial^2 P}{\partial y^2} = \frac{\partial^2 \mathrm{X}}{\partial x^2} - \frac{\partial^2 \mathrm{X}}{\partial y^2} + 2\frac{\partial^2 \mathrm{Y}}{\partial x \partial y} + \frac{\partial T_x}{\partial x} + \frac{\partial T_y}{\partial y}. \tag{S22}$$

### B. Linear stability analysis

The homogeneous steady state of active smectic layers reads: $m = m_H$, $\boldsymbol{k} = \hat{\boldsymbol{y}}$, $n = n_H$ with $n_H \triangleq 2\sqrt{\beta/\alpha}$, and $\boldsymbol{v} = \boldsymbol{0}$. Next, we analyze the stability of such a homogeneous steady state. The perturbation equations read:

$$\begin{aligned} \frac{\partial \delta M_x}{\partial t} =& D_m\frac{\partial^2 \delta m}{\partial x \partial y} + D_n\left(\frac{\partial^2 \delta M_x}{\partial y^2} - \frac{\partial^2 \delta M_y}{\partial x \partial y}\right) - \widetilde{\lambda}_m\left(\frac{\partial^2 \delta k_x}{\partial x^2} + \frac{\partial^2 \delta k_y}{\partial x \partial y}\right) \\ &- \xi_m\left(\frac{\partial^4 \delta k_x}{\partial x^4} + \frac{\partial^4 \delta k_x}{\partial x^2 \partial y^2} + \frac{\partial^4 \delta k_y}{\partial x^3 \partial y} + \frac{\partial^4 \delta k_y}{\partial x \partial y^3}\right) - d\frac{\partial^2 \delta n}{\partial x \partial y} - m_H\frac{\partial \delta v_y}{\partial x}, \end{aligned} \tag{S23}$$

$$\begin{aligned} \frac{\partial \delta M_y}{\partial t} =& -\nu n_H \delta m + D_m\frac{\partial^2 \delta m}{\partial y^2} + D_n\left(\frac{\partial^2 \delta M_y}{\partial x^2} - \frac{\partial^2 \delta M_x}{\partial x \partial y}\right) - \widetilde{\lambda}_m\left(\frac{\partial^2 \delta k_x}{\partial x \partial y} + \frac{\partial^2 \delta k_y}{\partial y^2}\right) \\ &- \xi_m\left(\frac{\partial^4 \delta k_x}{\partial x^3 \partial y} + \frac{\partial^4 \delta k_x}{\partial x \partial y^3} + \frac{\partial^4 \delta k_y}{\partial x^2 \partial y^2} + \frac{\partial^4 \delta k_y}{\partial y^4}\right) - d\frac{\partial^2 \delta n}{\partial y^2} - m_H\frac{\partial \delta v_y}{\partial y}, \end{aligned} \tag{S24}$$

$$\frac{\partial \delta n}{\partial t} = D_n\left(\frac{\partial^2 \delta n}{\partial x^2} + \frac{\partial^2 \delta n}{\partial y^2}\right) - \alpha n_H \delta n, \tag{S25}$$

$$-\lambda \delta v_y + \eta \nabla^2 \delta v_y = \frac{\partial \delta P}{\partial y} + \frac{\partial \delta \mathrm{X}}{\partial y} - \frac{\partial \delta \mathrm{Y}}{\partial x} - \delta T_y, \tag{S26}$$

$$\nabla^2 \delta P = \frac{\partial^2 \delta \mathrm{X}}{\partial x^2} - \frac{\partial^2 \delta \mathrm{X}}{\partial y^2} + 2\frac{\partial^2 \delta \mathrm{Y}}{\partial x \partial y} + \frac{\partial \delta T_x}{\partial x} + \frac{\partial \delta T_y}{\partial y}, \tag{S27}$$

where we defined (as in the main text),

$$\widetilde{\lambda}_m = \lambda_m + \nu_K n_H = \lambda_m + 2\nu_K\sqrt{\frac{\beta}{\alpha}}, \tag{S28}$$

which is a modified activity parameter, which collects the effects of the parameters $\alpha$, $\beta$, and $\nu_K$. Since

$$\delta m = \delta\left(\sqrt{\boldsymbol{M}\cdot\boldsymbol{M}}\right) = \delta M_y \quad , \quad \delta\boldsymbol{k} = \delta\left(\frac{\boldsymbol{M}}{m}\right) = \frac{1}{m_H}\delta M_x\hat{\boldsymbol{x}} \quad \Rightarrow \quad \delta k_x = \frac{1}{m_H}\delta M_x \quad , \quad \delta k_y = 0, \tag{S29}$$

we find that the perturbations to the quantities defined in Eq. (S20) read

$$\begin{aligned}
\delta\mathrm{X} &= \frac{B}{2m_H}\delta m - K\left(\frac{\partial^2\delta k_x}{\partial x\partial y} + \frac{\partial^2\delta k_y}{\partial y^2}\right) = \frac{B}{2m_H}\delta M_y - \frac{K}{m_H}\frac{\partial^2\delta M_x}{\partial x\partial y},\\
\delta\mathrm{Y} &= -B\frac{m_H - m_S}{m_H}\delta k_x + K\left(\frac{\partial^2\delta k_x}{\partial x^2} + \frac{\partial^2\delta k_y}{\partial x\partial y}\right) = -B\frac{m_H - m_S}{m_H^2}\delta M_x + \frac{K}{m_H}\frac{\partial^2\delta M_x}{\partial x^2},\\
\delta T_x &= -\zeta_b\frac{\partial\delta k_x}{\partial y} - \chi\frac{\partial\delta m}{\partial x} = -\frac{\zeta_b}{m_H}\frac{\partial\delta M_x}{\partial y} - \chi\frac{\partial\delta M_y}{\partial x},\\
\delta T_y &= -\zeta_s\left(\frac{\partial\delta k_x}{\partial x} + \frac{\partial\delta k_y}{\partial y}\right) - \zeta_b\frac{\partial\delta k_y}{\partial y} - \chi\frac{\partial\delta m}{\partial y} = -\frac{\zeta_s}{m_H}\frac{\partial\delta M_x}{\partial x} - \chi\frac{\partial\delta M_y}{\partial y},
\end{aligned} \tag{S30}$$

Given these perturbations, the resulting perturbation equations on the smectic director field can be expressed as:

$$\frac{\partial\delta M_x}{\partial t} = -\frac{\widetilde{\lambda}_m}{m_H}\frac{\partial^2\delta M_x}{\partial x^2} + D_n\frac{\partial^2\delta M_x}{\partial y^2} - \frac{\xi_m}{m_H}\frac{\partial^4\delta M_x}{\partial x^4} - \frac{\xi_m}{m_H}\frac{\partial^4\delta M_x}{\partial x^2\partial y^2} + (D_m - D_n)\frac{\partial^2\delta M_y}{\partial x\partial y} - d\frac{\partial^2\delta n}{\partial x\partial y} - m_H\frac{\partial\delta v_y}{\partial x}, \tag{S31}$$

and

$$\begin{aligned}
\frac{\partial\delta M_y}{\partial t} =& -\left(D_n + \frac{\widetilde{\lambda}_m}{m_H}\right)\frac{\partial^2\delta M_x}{\partial x\partial y} - \frac{\xi_m}{m_H}\frac{\partial^4\delta M_x}{\partial x^3\partial y} - \frac{\xi_m}{m_H}\frac{\partial^4\delta M_x}{\partial x\partial y^3} - \nu n_H\delta M_y + D_n\frac{\partial^2\delta M_y}{\partial x^2} + D_m\frac{\partial^2\delta M_y}{\partial y^2}\\
&- d\frac{\partial^2\delta n}{\partial y^2} - m_H\frac{\partial\delta v_y}{\partial y},
\end{aligned} \tag{S32}$$

The perturbation to the net number density of dislocations then read:

$$\frac{\partial\delta n}{\partial t} = -\alpha n_H\delta n + D_n\nabla^2\delta n, \tag{S33}$$

The perturbation on the force balance equation read:

$$-\lambda\delta v_y + \eta\nabla^2\delta v_y = \frac{\partial\delta P}{\partial y} + \left(\frac{\zeta_s}{m_H} + B\frac{m_H - m_S}{m_H^2}\right)\frac{\partial\delta M_x}{\partial x} - \frac{K}{m_H}\frac{\partial^3\delta M_x}{\partial x^3} - \frac{K}{m_H}\frac{\partial^3\delta M_x}{\partial x\partial y^2} + \left(\chi + \frac{B}{2m_H}\right)\frac{\partial\delta M_y}{\partial y}, \tag{S34}$$

and

$$\begin{aligned}
\nabla^2\delta P =& -\left(\frac{\zeta_s + \zeta_b}{m_H} + 2B\frac{m_H - m_S}{m_H^2}\right)\frac{\partial^2\delta M_x}{\partial x\partial y} + \frac{K}{m_H}\frac{\partial^4\delta M_x}{\partial x^3\partial y} + \frac{K}{m_H}\frac{\partial^4\delta M_x}{\partial x\partial y^3}\\
&+ \left(-\chi + \frac{B}{2m_H}\right)\frac{\partial^2\delta M_y}{\partial x^2} - \left(\chi + \frac{B}{2m_H}\right)\frac{\partial^2\delta M_y}{\partial y^2}.
\end{aligned} \tag{S35}$$

In the Fourier space, these perturbation equations read:

$$\frac{\partial\widetilde{\delta M_x}}{\partial t} = \left(\frac{\widetilde{\lambda}_m}{m_H}q_x^2 - D_n q_y^2 - \frac{\xi_m}{m_H}q^2 q_x^2\right)\widetilde{\delta M_x} - (D_m - D_n)\, q_x q_y\widetilde{\delta M_y} + d q_x q_y\widetilde{\delta n} - \mathrm{i}m_H q_x\widetilde{\delta v_y}, \tag{S36}$$

$$\frac{\partial\widetilde{\delta M_y}}{\partial t} = \left(D_n + \frac{\widetilde{\lambda}_m}{m_H} - \frac{\xi_m}{m_H}q^2\right)q_x q_y\widetilde{\delta M_x} - \left(\nu n_H + D_n q_x^2 + D_m q_y^2\right)\widetilde{\delta M_y} + d q_y^2\widetilde{\delta n} - \mathrm{i}m_H q_y\widetilde{\delta v_y}, \tag{S37}$$

and

$$\frac{\partial\widetilde{\delta n}}{\partial t} = -\left(\alpha n_H + D_n q^2\right)\widetilde{\delta n}, \tag{S38}$$

while

$$\widetilde{\delta v_y} = -\mathrm{i}\frac{q_y}{(\lambda+\eta q^2)}\widetilde{\delta P} - \mathrm{i}\left(\frac{\zeta_s}{m_H} + B\frac{m_H - m_S}{m_H^2} + \frac{K}{m_H}q^2\right)\frac{q_x}{(\lambda+\eta q^2)}\widetilde{\delta M_x} - \mathrm{i}\left(\chi + \frac{B}{2m_H}\right)\frac{q_y}{(\lambda+\eta q^2)}\widetilde{\delta M_y}, \tag{S39}$$

and

$$\widetilde{\delta P} = -\left[\frac{\zeta_s+\zeta_b}{m_H} + 2B\frac{m_H - m_S}{m_H^2} + \frac{K}{m_H}q^2\right]\frac{q_x q_y}{q^2}\widetilde{\delta M_x} + \left[-\chi + \frac{B}{2m_H}\frac{(q_x^2 - q_y^2)}{q^2}\right]\widetilde{\delta M_y}, \tag{S40}$$

where $q = |\boldsymbol{q}|$ with $\boldsymbol{q} = (q_x, q_y)$ being the wavevector; $\widetilde{\delta M_x}$, $\widetilde{\delta M_y}$, $\widetilde{\delta n}$, $\widetilde{\delta v_x}$, $\widetilde{\delta v_y}$, and $\widetilde{\delta P}$ are the Fourier transforms of $\delta M_x(\boldsymbol{x})$, $\delta M_y(\boldsymbol{x})$, $\delta n(\boldsymbol{x})$, $\delta v_x(\boldsymbol{x})$, $\delta v_y(\boldsymbol{x})$, and $\delta P(\boldsymbol{x})$, respectively.

Substituting Eq. (S40) into Eq. (S39), we obtain

$$\widetilde{\delta v_y} = -\mathrm{i}\left(\frac{\zeta_s}{m_H}\frac{q_x^2}{q^2} - \frac{\zeta_b}{m_H}\frac{q_y^2}{q^2} + B\frac{m_H - m_S}{m_H^2}\frac{q_x^2 - q_y^2}{q^2} + \frac{K}{m_H}q_x^2\right)\frac{q_x}{(\lambda+\eta q^2)}\widetilde{\delta M_x} - \mathrm{i}\frac{B}{m_H}\frac{q_x^2}{q^2}\frac{q_y}{(\lambda+\eta q^2)}\widetilde{\delta M_y}. \tag{S41}$$

*Jacobian expression* – Since $\alpha > 0$, $n_H > 0$ and $D_n > 0$, Eq. (S38) suggests that the perturbation in $\delta n$ cannot grow. Therefore, we focus on perturbations relative to the smectic director, and set $\delta n = 0$.

Substituting Eqs. (S41) into Eqs. (S36) and (S37), we get

$$\frac{\partial}{\partial t}\begin{pmatrix}\widetilde{\delta M_x}\\ \widetilde{\delta M_y}\end{pmatrix} = \boldsymbol{G}\cdot\begin{pmatrix}\widetilde{\delta M_x}\\ \widetilde{\delta M_y}\end{pmatrix}, \tag{S42}$$

where the components of the Jacobian matrix $\boldsymbol{G}(\boldsymbol{q}) = [G_{ij}(\boldsymbol{q})]_{2\times 2}$ read

$$\begin{aligned} G_{11} = &\left(\frac{\widetilde{\lambda}_m}{m_H} - \frac{\xi_m}{m_H}q^2\right)q^2\cos^2\phi - D_n q^2\sin^2\phi \\ &+ \left[-\left(\zeta_s + B\frac{m_H - m_S}{m_H} + Kq^2\right)\cos^2\phi + \left(\zeta_b + B\frac{m_H - m_S}{m_H}\right)\sin^2\phi\right]\frac{q^2\cos^2\phi}{(\lambda+\eta q^2)}, \end{aligned} \tag{S43}$$

$$G_{12} = -\left[D_m - D_n + B\frac{1}{(\lambda+\eta q^2)}\cos^2\phi\right]q^2\sin\phi\cos\phi, \tag{S44}$$

$$G_{21} = \left\{\begin{aligned} &D_n + \frac{\widetilde{\lambda}_m}{m_H} - \frac{\xi_m}{m_H}q^2 \\ &+ \frac{1}{(\lambda+\eta q^2)}\left[-\left(\zeta_s + B\frac{m_H - m_S}{m_H} + Kq^2\right)\cos^2\phi + \left(\zeta_b + B\frac{m_H - m_S}{m_H}\right)\sin^2\phi\right]\end{aligned}\right\}q^2\sin\phi\cos\phi, \tag{S45}$$

$$G_{22} = -\left[\nu n_H + D_n q^2\cos^2\phi + D_m q^2\sin^2\phi + B\frac{q^2}{(\lambda+\eta q^2)}\sin^2\phi\cos^2\phi\right], \tag{S46}$$

where $\phi = \arg(\boldsymbol{q})$ is the argument of the wavevector $\boldsymbol{q}$. The eigenvalues $\boldsymbol{\omega}$ (i.e., the growth rate of perturbations) of $\boldsymbol{G}$ determine the stability of the homogeneous state. The characteristic equation reads:

$$\omega^2 + b(\boldsymbol{q})\omega + c(\boldsymbol{q}) = 0, \tag{S47}$$

where $b(\boldsymbol{q}) = -\mathrm{tr}(\boldsymbol{G})$ and $c(\boldsymbol{q}) = \det(\boldsymbol{G})$; the solution of the characteristic equation are

$$\omega_\pm(\boldsymbol{q}) = \frac{1}{2}\left(-b(\boldsymbol{q}) \pm \sqrt{b(\boldsymbol{q})^2 - 4c(\boldsymbol{q})}\right), \tag{S48}$$

With the expressions of $G_{ij}$ (Eqs. (S43)–(S46)), we obtain

$$\begin{aligned} b(\boldsymbol{q}) = &\,\nu n_H + D_n q^2 + D_m q^2\sin^2\phi + B\frac{q^2\sin^2\phi\cos^2\phi}{(\lambda+\eta q^2)} + \left(-\frac{\widetilde{\lambda}_m}{m_H} + \frac{\xi_m}{m_H}q^2\right)q^2\cos^2\phi \\ &+ \frac{q^2\cos^2\phi}{(\lambda+\eta q^2)}\left[\left(\zeta_s + B\frac{m_H - m_S}{m_H} + Kq^2\right)\cos^2\phi - \left(\zeta_b + B\frac{m_H - m_S}{m_H}\right)\sin^2\phi\right], \end{aligned} \tag{S49}$$

$$c(\boldsymbol{q}) = \left(\nu n_H + D_n q^2\right) q^2 \cos^2\phi \left\{ \begin{aligned} & -\frac{\tilde{\lambda}_m}{m_H} + \frac{\xi_m}{m_H} q^2 \\ & + \frac{1}{(\lambda + \eta q^2)} \left[ \left( \zeta_s + B\frac{m_H - m_S}{m_H} + K q^2 \right) \cos^2\phi - \left( \zeta_b + B\frac{m_H - m_S}{m_H} \right) \sin^2\phi \right] \end{aligned} \right\}$$
$$+ D_n q^2 \sin^2\phi \left[ \nu n_H + D_m q^2 + B\frac{q^2 \cos^2\phi}{(\lambda + \eta q^2)} \right]. \tag{S50}$$

The stability condition for the homogeneous steady state requires:

$$\mathrm{Re}\left[\omega_\pm(\boldsymbol{q})\right] < 0 \quad \Leftrightarrow \quad \begin{cases} b(\boldsymbol{q}) > 0 \\ c(\boldsymbol{q}) > 0 \end{cases} \tag{S51}$$

for all wavevector $\boldsymbol{q}$.

### 1. *Specific role of $\tilde{\lambda}_m$: stability requirement in the passive case*

In the passive limit $\zeta_s = \zeta_b = 0$, $\chi = 0$, $m_S = m_H$, we find that:

$$c(\boldsymbol{q}) = D_n \left[ D_m \sin^2\phi + \left( -\frac{\tilde{\lambda}_m}{m_H} + \frac{\xi_m}{m_H} q^2 \right) \cos^2\phi + \left( B \sin^2\phi + K q^2 \cos^2\phi \right) \frac{\cos^2\phi}{(\lambda + \eta q^2)} \right] q^4. \tag{S52}$$

In the limit $q \to 0$ and $\phi \to 0$, the condition of $c(\boldsymbol{q}) > 0$ implies that

$$\tilde{\lambda}_m < 0. \tag{S53}$$

which, in the limit $n_H = 0$ (or $\nu_K = 0$), is equivalent to $\lambda_m < 0$.

### 2. *Specific role of $\nu_K$: stability requirement in the passive case*

Here we consider the specific role of the compression-induced motility of dislocations, $\nu$, by setting all other activity parameters to be zero ($\zeta_s = 0$, $\zeta_b = 0$, $\chi = 0$, $m_S = m_H$) and $\nu_K = 0$. Consequently, we have

$$b(\boldsymbol{q}) = \nu n_H + D_n q^2 + D_m q^2 \sin^2\phi + \left( -\frac{\lambda_m}{m_H} + \frac{\xi_m}{m_H} q^2 \right) q^2 \cos^2\phi + \left( B \sin^2\phi + K q^2 \cos^2\phi \right) \frac{q^2 \cos^2\phi}{(\lambda + \eta q^2)}, \tag{S54}$$

$$c\left(\boldsymbol{q}\right) = \nu n_H q^2 \left[ D_n \sin^2\phi + \left( -\frac{\lambda_m}{m_H} + \frac{\xi_m}{m_H} q^2 \right) \cos^2\phi + K q^2 \frac{\cos^4\phi}{(\lambda + \eta q^2)} \right]$$
$$+ D_n q^4 \left[ D_m \sin^2\phi + \left( -\frac{\lambda_m}{m_H} + \frac{\xi_m}{m_H} q^2 \right) \cos^2\phi + \left( B \sin^2\phi + K q^2 \cos^2\phi \right) \frac{\cos^2\phi}{(\lambda + \eta q^2)} \right]. \tag{S55}$$

In particular, $c(q \to 0) \sim \nu n_H (D_n \sin^2\phi - \lambda_m / m_H \cos^2\phi) q^2$. Thus, $\nu < 0$ will lead to large-scale instabilities; in such a case, numerical simulations diverge. In our study here, we set $\nu \geq 0$.

### 3. *General case: small-scale stability in arbitrary directions*

We first consider small-scale perturbations, i.e., $q \to +\infty$. The leading-order terms in $b(q)$ and $c(q)$ read:

$$b\left(q \to \infty\right) \simeq \frac{\xi_m}{m_H} q^4 \cos^2\phi > 0, \tag{S56}$$

$$c\left(q \to \infty\right) \simeq \frac{\xi_m}{m_H} D_n q^6 \cos^2\phi > 0. \tag{S57}$$

This suggests the active smectic system is stable at small scales when $\xi_m > 0$.

In particular, when $\xi_m = 0$, we have

$$b\,(q \to \infty) \simeq \left[D_n + D_m - \left(D_m + \frac{\widetilde{\lambda}_m}{m_H}\right)\cos^2\phi + \frac{K}{\eta}\cos^4\phi\right] q^2, \tag{S58}$$

$$c\,(q \to \infty) \simeq D_n \left[D_m - \left(D_m + \frac{\widetilde{\lambda}_m}{m_H}\right)\cos^2\phi + \frac{K}{\eta}\cos^4\phi\right] q^4. \tag{S59}$$

The stability requirement Eq. (S51) results in an up limit of the rescaled parameter $\widetilde{\lambda}_m$:

$$\widetilde{\lambda}_m^\star = \begin{cases} m_H\left(2\sqrt{\dfrac{D_m K}{\eta}} - D_m\right) & , \quad D_m < \dfrac{K}{\eta} \\ \dfrac{K m_H}{\eta} & , \quad D_m > \dfrac{K}{\eta} \end{cases} \tag{S60}$$

When $\widetilde{\lambda}_m > \widetilde{\lambda}_m^\star$, the active smectic layers become unstable at small scales; correspondingly, numerical simulations diverge. Equivalently, Eq. (S60) corresponds to an up limit of the dislocation creation rate:

$$\beta^\star = \alpha \frac{(\widetilde{\lambda}_m^\star - \lambda_m)^2}{4\nu_K^2}, \tag{S61}$$

where $\widetilde{\lambda}_m^\star$ is given by Eq. (S60).

#### 4. General case: large-scale stability in arbitrary directions

We next consider large-scale perturbations, i.e., $q \to 0$. The leading-order expansions of $b$ and $c$ are

$$b\,(q \to 0) \simeq \nu n_H > 0, \tag{S62}$$

and

$$c\,(q \to 0) \simeq \nu n_H \left\{\frac{1}{\lambda}\left(\zeta_s + \zeta_b + 2B\frac{m_H - m_S}{m_H}\right)\cos^4\phi - \left[D_n + \frac{\widetilde{\lambda}_m}{m_H} + \frac{1}{\lambda}\left(\zeta_b + B\frac{m_H - m_S}{m_H}\right)\right]\cos^2\phi + D_n\right\} q^2. \tag{S63}$$

The stability of active smectic layers at large scales requires:

$$\left(\zeta_s + \zeta_b + 2B\frac{m_H - m_S}{m_H}\right)\cos^4\phi - \left[\lambda D_n + \frac{\lambda\widetilde{\lambda}_m}{m_H} + \left(\zeta_b + B\frac{m_H - m_S}{m_H}\right)\right]\cos^2\phi + \lambda D_n > 0 \quad (\forall\phi)\,. \tag{S64}$$

which leads to constraints on the parameters. The detailed expression is complicated. Indeed, we have the following sufficient conditions to enforce the stability of active smectic layers at large scales,

$$\begin{cases} -\dfrac{\widetilde{\lambda}_m}{m_H} - \dfrac{1}{\lambda}\left(\zeta_b + B\dfrac{m_H - m_S}{m_H}\right) > 0 \\ \zeta_s + \zeta_b + 2B\dfrac{m_H - m_S}{m_H} > 0 \end{cases} \quad \Leftrightarrow \quad -\zeta_s - 2B\frac{m_H - m_S}{m_H} < \zeta_b < -\frac{\lambda\widetilde{\lambda}_m}{m_H} - B\frac{m_H - m_S}{m_H}. \tag{S65}$$

This suggests that when the active bend traction $\zeta_b$ is bounded between $\zeta_{b,1} = -\zeta_s - 2B(m_H - m_S)/m_H$ and $\zeta_{b,2} = -\lambda\widetilde{\lambda}_m/m_H - B(m_H - m_S)/m_H$, active smectic layers are stable under large-scale perturbations.

### 5. General case: stability along the smectic layers direction

*Stability along the smectic layers.* – We here consider the perturbations along the smectic layers, i.e., $\phi = 0$,

$$b = \nu n_H + \left(D_n - \frac{\widetilde{\lambda}_m}{m_H}\right) q^2 + \frac{\xi_m}{m_H} q^4 + \frac{q^2}{(\lambda + \eta q^2)} \left(\zeta_s + B\frac{m_H - m_S}{m_H} + Kq^2\right), \tag{S66}$$

$$c = \left(\nu n_H + D_n q^2\right)\left[-\frac{\widetilde{\lambda}_m}{m_H} + \frac{\xi_m}{m_H} q^2 + \frac{1}{(\lambda + \eta q^2)} \left(\zeta_s + B\frac{m_H - m_S}{m_H} + Kq^2\right)\right] q^2. \tag{S67}$$

The stability condition Eq. (S51) reads:

$$\zeta_s + B\frac{m_H - m_S}{m_H} - \frac{\widetilde{\lambda}_m \lambda}{m_H} + \left(K + \frac{\xi_m \lambda - \widetilde{\lambda}_m \eta}{m_H}\right) q^2 + \frac{\xi_m}{m_H} \eta q^4 > 0 \qquad (\forall q), \tag{S68}$$

which further leads to,

$$\widetilde{\lambda}_m < \min\left\{\frac{1}{\lambda}\left[\zeta_s m_H + B\left(m_H - m_S\right)\right], \frac{1}{\eta}\left(K m_H + \xi_m \lambda\right)\right\}, \tag{S69}$$

or

$$\begin{cases} \zeta_s > -B\dfrac{(m_H - m_S)}{m_H} + \dfrac{\lambda}{\eta}K + \dfrac{\xi_m \lambda^2}{\eta m_H} \\ \dfrac{1}{\eta}\left(K m_H + \xi_m \lambda\right) < \widetilde{\lambda}_m < \dfrac{1}{\eta}\left(K m_H - \xi_m \lambda\right) + 2\sqrt{\dfrac{\xi_m}{\eta}\left[\zeta_s m_H + B\left(m_H - m_S\right) - \dfrac{\lambda}{\eta} K m_H\right]} \end{cases} \tag{S70}$$

*Critical $\zeta_s$.* Equations (S69) and (S70) result in a critical active splay traction,

$$\zeta_s^{\rm cr} = -B\frac{(m_H - m_S)}{m_H} + \frac{\lambda}{m_H} \min\left\{\widetilde{\lambda}_m, \frac{K m_H + \xi_m \lambda}{\eta}\right\}. \tag{S71}$$

Defining the quantities:

$$\zeta_s^* = -B\frac{(m_H - m_S)}{m_H} + \frac{\lambda \widetilde{\lambda}_m}{m_H}, \tag{S72}$$

$$\zeta_s^\diamond = -B\frac{(m_H - m_S)}{m_H} + K\frac{\lambda}{\eta} + \frac{\xi_m \lambda^2}{m_H \eta}. \tag{S73}$$

Eq. (S71) then reads

$$\zeta_s^{\rm cr} = \min\left\{\zeta_s^*, \zeta_s^\diamond\right\}, \tag{S74}$$

as discussed in the main text. The active smectic layers will undergo buckling instability when $\zeta_s < \zeta_s^{\rm cr}$. Note that, in general, $\zeta_s^{\rm cr} \le \zeta_s^*$ and $\zeta_s^{\rm cr} \le \zeta_s^\diamond$: when $\widetilde{\lambda}_m < (K m_H + \xi_m \lambda)/\eta$, $\zeta_s^{\rm cr} = \zeta_s^* < \zeta_s^\diamond$; while when $\widetilde{\lambda}_m > (K m_H + \xi_m \lambda)/\eta$, $\zeta_s^{\rm cr} = \zeta_s^\diamond < \zeta_s^*$. In agreement with our theoretical predictions, in our numerical simulations, steady state flows occur as soon as $\zeta_s <_s^{\rm cr}$; see Fig. S1.

*Critical $\widetilde{\lambda}_m$.* Equations (S69) and (S70) also results in a critical value of $\widetilde{\lambda}_m$:

$$\widetilde{\lambda}_m^{\rm cr} = \begin{cases} \dfrac{1}{\lambda}\left[\zeta_s m_H + B\left(m_H - m_S\right)\right] \quad , \quad \zeta_s < -B\dfrac{(m_H - m_S)}{m_H} + \dfrac{\lambda}{\eta}K + \dfrac{\xi_m \lambda^2}{\eta m_H} \\ \dfrac{1}{\eta}\left(K m_H - \xi_m \lambda\right) + 2\sqrt{\dfrac{\xi_m}{\eta}\left[\zeta_s m_H + B\left(m_H - m_S\right) - \dfrac{\lambda}{\eta} K m_H\right]} \quad , \quad \text{otherwise} \end{cases} \tag{S75}$$

beyond which the active smectic layers will undergo instability. The critical value $\widetilde{\lambda}_m^{\rm cr}$ equivalently corresponds to a critical dislocation creation rate, $\beta^{\rm cr} = \alpha(\widetilde{\lambda}_m^{\rm cr} - \lambda_m)^2/(4\nu_K^2)$, as well as a critical value of $\nu_K$, $\nu_K^{\rm cr} = (\widetilde{\lambda}_m^{\rm cr} - \lambda_m)/n_H$.

*Critical* $m_S$. When $m_S \neq m_H$, there are non-zero deviatoric stresses in the smectic layers even in the homogeneous steady state: $\sigma_{xx} = B(m_H - m_S)/(2m_H)$, $\sigma_{yy} = -B(m_H - m_S)/(2m_H)$, $\sigma_{xy} = \sigma_{yx} = 0$. In the case of $m_S > m_H$, $\sigma_{xx} < 0$, sufficiently large compressive stress along the smectic layers can lead to bucking instability. Equations (S69) and (S70) lead to a critical value of $m_S$:

$$m_S^{\rm cr} = m_H + \frac{\zeta_s m_H}{B} - \frac{\lambda}{B}\min\left\{\widetilde{\lambda}_m, \frac{K m_H + \xi_m \lambda}{\eta}\right\}. \tag{S76}$$

In particular, in the absence of activity parameters and no dislocations, $m_S^{\rm cr} = m_H - \lambda\lambda_m/B \ > m_H$; the corresponding critical compressive stress that leads to buckling instability is, $\sigma_{xx}^{\rm cr} = \lambda\lambda_m/m_H \ < 0$. The numerical evaluation of $\omega$ shows that $\omega \sim 0$ for $m_S = m_S^{\rm cr}$, see Fig. S2.

*Critical dislocation motilities.* As discussed in the main text, both the compression-induced motility $\nu$ and the splay-induced motility $\nu_K$ of dislocations can lead to flows, see Figs. S3, S4 and S5.

*Characteristic wavenumber* $q_c$ *of buckling.* The characteristic wavenumber (denoted $q_c$) for such buckling instability corresponds to the wavenumber that maximizes ${\rm Re}[\omega(q)]$. When the buckling instability occurs, $c(q) < 0$, thus $\omega_+ = (-b + \sqrt{b^2 - 4c})/2 > 0$ and $\omega_- = (-b - \sqrt{b^2 - 4c})/2 < 0$. The characteristic wavenumber $q_c$ can be obtained by letting ${\rm d}\omega_+/{\rm d}q = 0$. When the buckling instability occurs, i.e., $\zeta_s < \zeta_s^{\rm cr}$, we have a simplified expression of $\omega_+$ as:

$$\omega_+ = -\frac{\xi_m}{m_H}q^4 - \frac{q^2}{(\lambda + \eta q^2)}\left[\zeta_s - \zeta_s^* + \left(K - \frac{\widetilde{\lambda}_m}{m_H}\eta\right)q^2\right]. \tag{S77}$$

Letting ${\rm d}\omega_+/{\rm d}q = 0$ leads to:

$$2\xi_m\eta^2 q_c^6 + \eta(4\xi_m\lambda + K m_H - \eta\widetilde{\lambda}_m)q_c^4 + 2\lambda(\xi_m\lambda + K m_H - \eta\widetilde{\lambda}_m)q_c^2 + \lambda m_H(\zeta_s - \zeta_s^*) = 0. \tag{S78}$$

To derive a simple analytical expression of $q_c$ for the general case of $\lambda > 0$ and $\eta > 0$, we here ignore the higher-order terms ($q_c^4$ and $q_c^6$ terms) in Eq. (S78) and obtain an estimate of $q_c$ as:

$$q_c \approx \sqrt{\frac{m_H(\zeta_s^* - \zeta_s)}{2(\xi_m\lambda + K m_H - \eta\widetilde{\lambda}_m)}} = \sqrt{\frac{\lambda(\zeta_s^* - \zeta_s)}{2\eta(\zeta_s^\diamond - \zeta_s^*)}}. \tag{S79}$$

Note that this simplified expression for $q_c$ works well only for parameters near the buckling transition.

- In the absence of activity ($\zeta_s \to 0$ and $\widetilde{\lambda}_m \to 0$), Eq. (S79) simplifies to

$$q_c = \sqrt{\frac{B\,(m_S - m_H)}{2\,(\xi_m\lambda + K m_H)}}. \tag{S80}$$

  We check that $q_c = 0$ when $m_s = m_H$; this is expected since the system should be stable for all $q$ in this limit.

- In the limit of $\lambda \to 0$, i.e., zero friction case,

$$\omega_+ = -\frac{\xi_m}{m_H}q^4 - \left(\frac{K}{\eta} - \frac{\widetilde{\lambda}_m}{m_H}\right)q^2 + \frac{1}{\eta}\left(\zeta_s^* - \zeta_s\right), \tag{S81}$$

  and Eq. (S78) simplifies to,

$$q_c = \sqrt{\max\left\{\frac{\eta\widetilde{\lambda}_m - K m_H}{2\xi_m\eta}, 0\right\}}. \tag{S82}$$

  This means that, when $\widetilde{\lambda}_m < K m_H/\eta$, we have $q_c = 0$; the stability of the system is then set by the sign of $\omega_+(0)$, which itself is set by the sign of the difference $\zeta_s^* - \zeta_s$. Correspondingly, we observe shear flow patterns in simulations with a wavelength $L_c^{\rm sim} = L$ where $L$ is the size of the simulation box.

### 6. *General case: stability along the normal to the smectic layers direction*

Finally, we consider the wave perturbations perpendicular to the layers, that is, $\phi = \pi/2$. In this case,

$$b = \nu n_H + (D_n + D_m)\, q^2 > 0, \tag{S83}$$

$$c = D_n q^2 \left(\nu n_H + D_m q^2\right) > 0, \tag{S84}$$

which shows that the active smectic layers are stable along the normal direction.

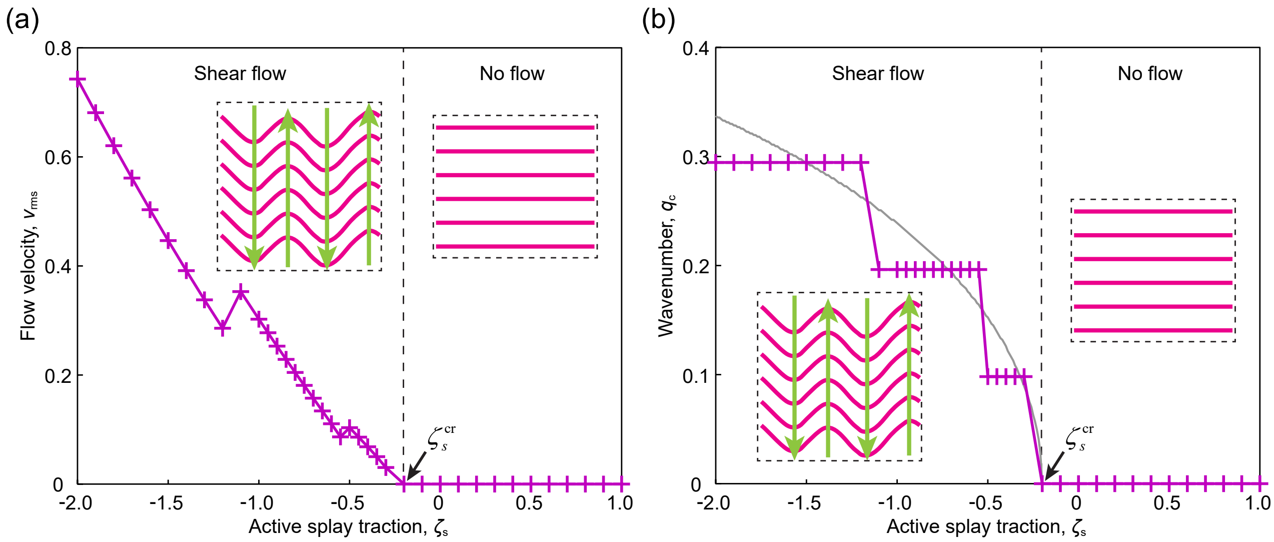


FIG. S1: Numerical simulations (magenta lines) exhibit a threshold to flows and pertubation wavevector that agree well our theoretical predictions. (a) The flow velocity, quantified by the root-mean-square velocity $v_{\rm rms}$, as a function of the active splay traction $\zeta_s$. Our linear stability analysis for an infinite system yields a critical value $\zeta_s^{\rm cr} = -0.2$ (dashed lines). (b) The wavenumber $q_c$ as a function of the active splay traction $\zeta_s$. Grey line: theoretical result for an infinite system predicted by Eq. (S78). Parameter values: $m_S = m_H = 1$, $\zeta_b = 0$, $\nu = 1$, $\nu_K = 0$, $\mu_d = 0$, $d = 0$, $\chi = 0$, $\xi_m = 0.5$.

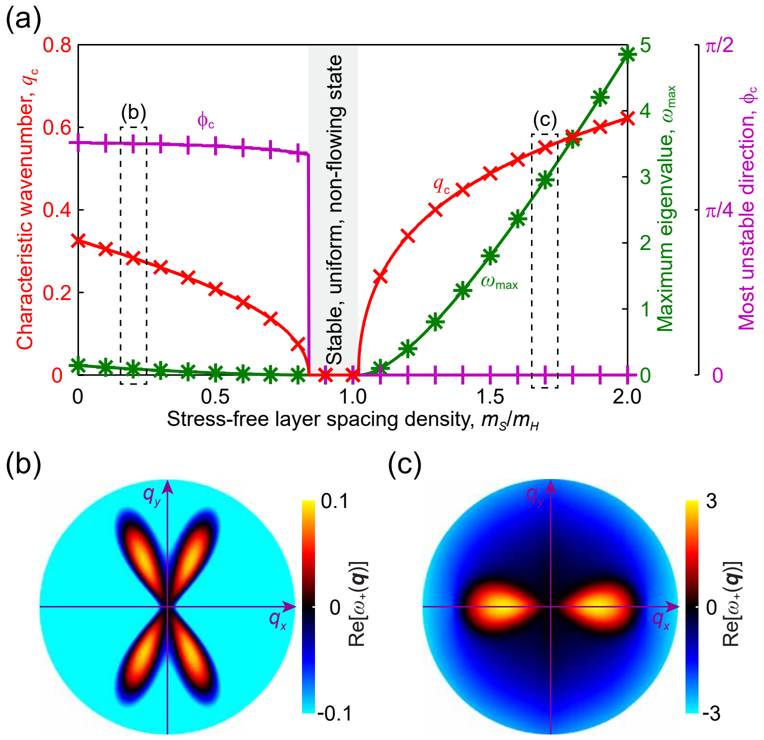


FIG. S2: Linear stability analysis of the uniform state. (a) The characteristic wavenumber $q_c$, the maximum eigenvalue $\omega_{\max}$, and the most unstable direction $\phi_c$ as functions of the stress-free layer spacing density $m_S$. Here, $q_c$, $\phi_c$, and $\omega_{\max}$ are determined by a numerical estimation of the maximum eigenvalue $\omega_+$ (as defined in Eq. (S48)) in the Fourier space $\boldsymbol{q}$. (b, c) Typical patterns of the real part of the eigenvalue $\mathrm{Re}[\omega_+(\boldsymbol{q})]$ in the Fourier space, corresponding to boxes shown in (a). Parameter values: $m_H = 1$, $\zeta_s = \zeta_b = 0$, $\nu = 1$, $\nu_K = 0$, $\xi_m = 0.5$.

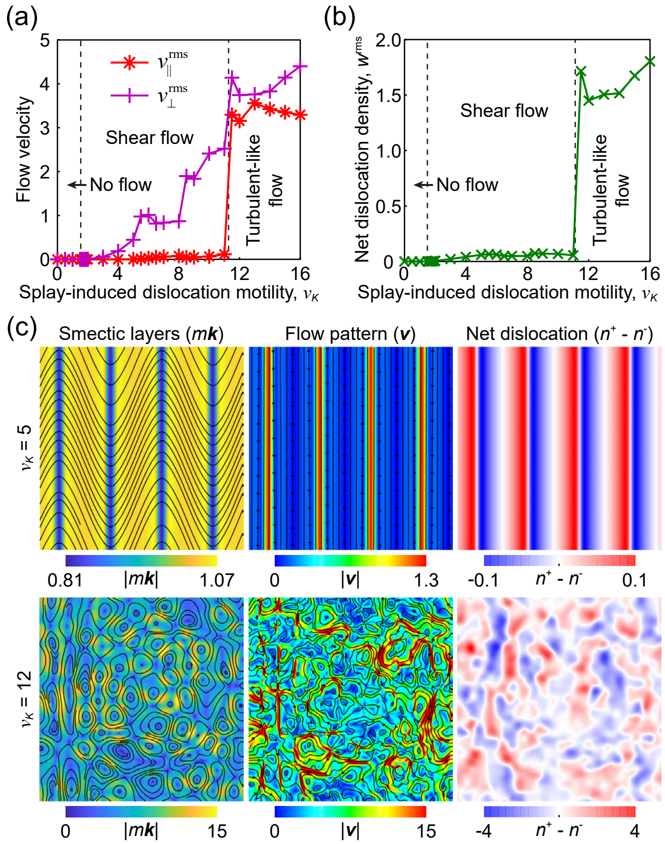


FIG. S3: The splay-induced motility of dislocations $\nu_K$ drives a continuous transition to flows in the absence of active tractions $\zeta_s = 0$. (a, b) The flow velocities (a) and the net dislocation density (b) as functions of the splay-induced dislocation motility. (c) Typical patterns at different levels of dislocation motilities: (*left*) smectic layers pattern; (*middle*) flow pattern; (*right*) net dislocation density field. Parameters: $m_S = m_H = 1$, $\zeta_s = \zeta_b = 0$, and $\beta = 0.1$.

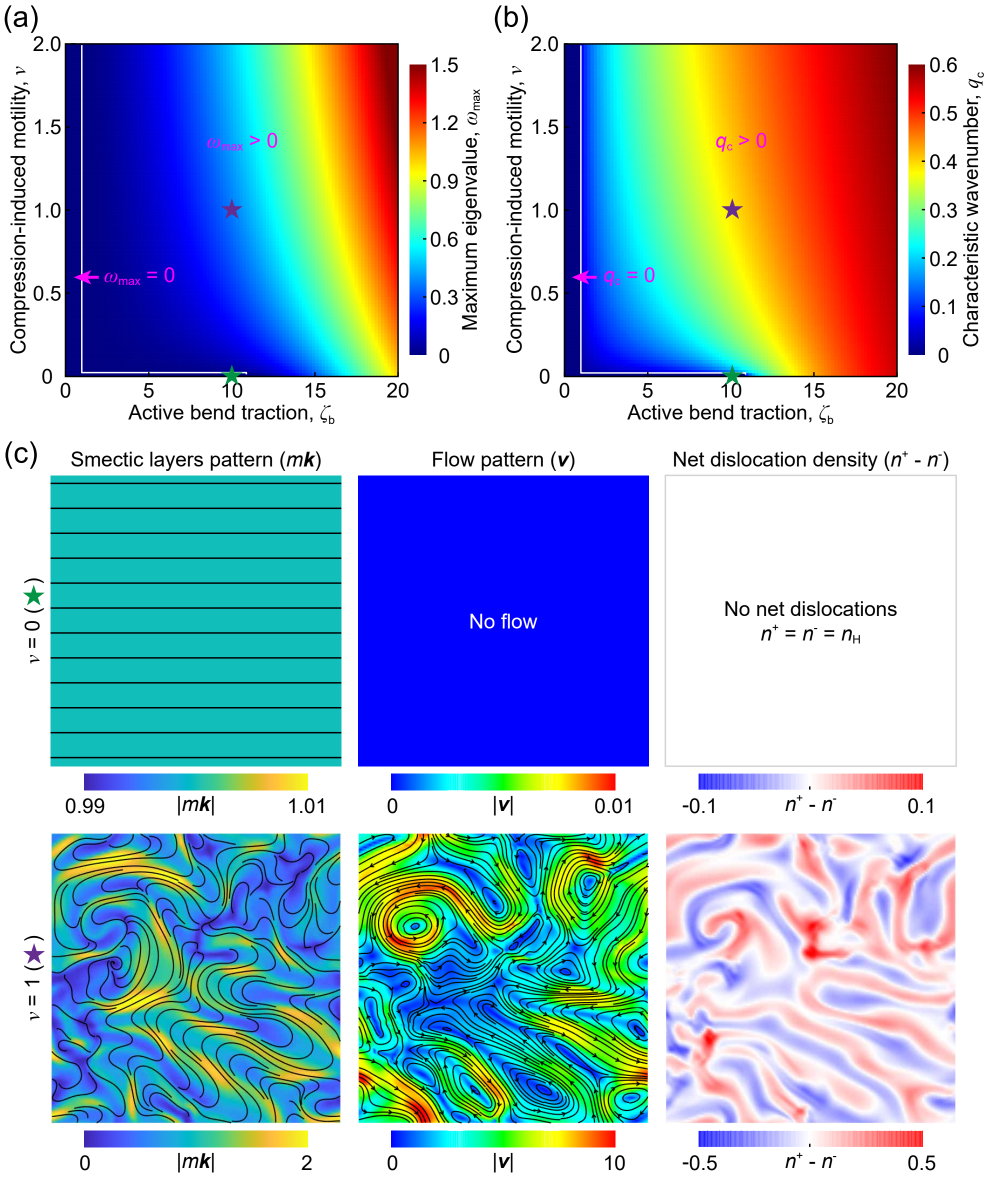


FIG. S4: The compression-induced motility of dislocations $\nu$ can lead to the onset of spontaneous flows in the presence of the active bend traction. (a, b) Analytical calculations of (a) the maximum eigenvalue $\omega_{\text{max}}$ and (b) the characteristic wavenumber $q_c$ with respect to the active bend traction $\zeta_b$ and the compression-induced motility of dislocations $\nu$. Symbols correspond to simulations shown in (c). (c) Typical patterns of active smectic layers at different levels of the compression-induced motility of dislocations where $\zeta_b = 10$. (*Left*) Smectic layers pattern: the color code represents the magnitude $m = |m\boldsymbol{k}|$, and black lines denote smectic layers. (*Middle*) Flow pattern: the color code represents the flow velocity magnitude $|\boldsymbol{v}|$, and the black lines with arrows denote streamlines. (*Right*) Net dislocation density field: the color code represents the net dislocation density $(n^+ - n^-)$. Parameters: $\zeta_s = 0$, $\nu_K = 0$, $\xi_m = 0.5$, $m_S = m_H = 1$, $\alpha = 1$, and $\beta = 0.1$.

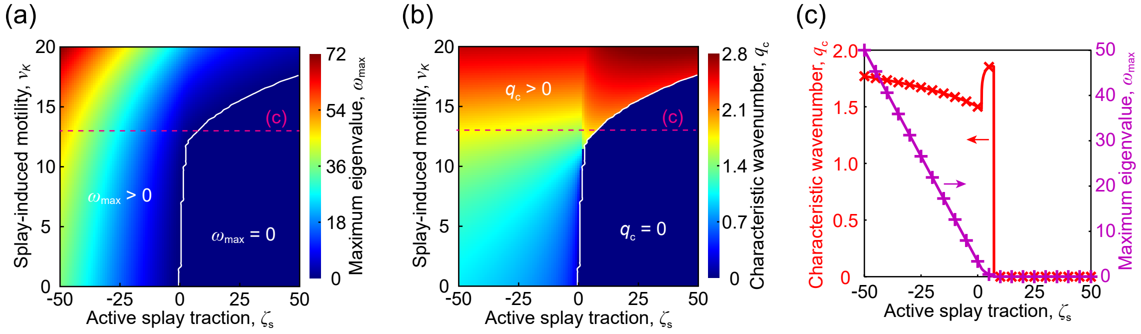


FIG. S5: The splay-induced motility of dislocations $\nu_K$ can lead to a discontinuous transition to flows in the presence of a sufficiently large active splay traction. Analytical calculations of (a) the maximum eigenvalue $\omega_{\max}$ and (b) the characteristic wavenumber $q_c$ with respect to the active splay traction $\zeta_s$ and the splay-induced motility of dislocations $\nu_K$. (c) The characteristic wavenumber $q_c$ and the maximum eigenvalue $\omega_{\max}$ as functions of the active splay traction $\zeta_s$ where $\nu_K = 13$; see the dashed lines in (a) and (b). Simulation results are presented in the main text, Fig. 5. Parameters: $\zeta_b = 0$, $\xi_m = 0.5$, $m_S = m_H = 1$, $\alpha = 1$, and $\beta = 0.1$.

## II. THEORY OF ACTIVE SMECTICS WITHOUT DISLOCATIONS

In this section, we focus on the case of no dislocations, i.e., $n^{\pm} \equiv 0$. In this case, the smectic director field ($m\boldsymbol{k}$) satisfies the no dislocation constraint: $\nabla \times (m\boldsymbol{k}) = \boldsymbol{0}$. In such a case, the smectic director field $m\boldsymbol{k}$ can be described by a scalar field, i.e., the displacement field normal to layers, denoted $u$, with the relationship: $m\boldsymbol{k} = m_H(\hat{\boldsymbol{y}} - \nabla u)$ [1, 2]. The dynamic equation of $\boldsymbol{M} = m\boldsymbol{k}$ then simplifies to $\partial_t u = J_m/m_H$ [1].

### A. Governing equations

In the absence of dislocations, i.e. $n^+ = n^- \equiv 0$, $n = w \equiv 0$. Consequently, the smectic director field $\boldsymbol{M}$ evolves as,

$$\frac{\partial \boldsymbol{M}}{\partial t} + \nabla J_m = \boldsymbol{0}. \tag{S85}$$

Besides, the smectic director field $\boldsymbol{M}$ satisfies $\nabla \times \boldsymbol{M} = \boldsymbol{0}$. Thus we can introduce a potential function $\Phi$, satisfying $\boldsymbol{M} = \nabla\Phi$. In particular, we set $\Phi = m_H(y-u)$, where $u$ is the displacement normal to the smectic layers (along the $y$ direction). Thus, we can express the smectic director field $m\boldsymbol{k}$ as a function of the displacement field $u$:

$$\boldsymbol{M} = m\boldsymbol{k} = m_H\left(\hat{\boldsymbol{y}} - \nabla u\right), \tag{S86}$$

$$\Rightarrow M_x = -m_H\frac{\partial u}{\partial x} \quad , \quad M_y = m_H\Big(1 - \frac{\partial u}{\partial y}\Big), \tag{S87}$$

which, in Cartesian coordinates, corresponds to:

$$\Rightarrow m = |\boldsymbol{M}| = m_H\sqrt{\left(\frac{\partial u}{\partial x}\right)^2 + \left(\frac{\partial u}{\partial y} - 1\right)^2} \quad , \quad k_x = \frac{-\dfrac{\partial u}{\partial x}}{\sqrt{1 - 2\dfrac{\partial u}{\partial y} + (\nabla u)^2}} \quad , \quad k_y = \frac{1 - \dfrac{\partial u}{\partial y}}{\sqrt{1 - 2\dfrac{\partial u}{\partial y} + (\nabla u)^2}}. \tag{S88}$$

Submitting Eq. (S86) into Eq. (S85), we get

$$\nabla\Big(-m_H\frac{\partial u}{\partial t} + J_m\Big) = \boldsymbol{0} \quad \Rightarrow \quad \frac{\partial u}{\partial t} = \frac{J_m}{m_H} = \frac{1}{m_H}m\boldsymbol{v}\cdot\boldsymbol{k} - \frac{D_m}{m_H}\boldsymbol{k}\cdot\nabla m + \frac{\lambda_m}{m_H}\nabla\cdot\boldsymbol{k} + \frac{\xi_m}{m_H}\nabla^2\left(\nabla\cdot\boldsymbol{k}\right), \tag{S89}$$

that is,

$$\begin{aligned}\frac{\partial u}{\partial t} = &\frac{1}{m_H}\left(v_x M_x + v_y M_y\right) + D_m\left(\frac{\partial^2 u}{\partial x^2} + \frac{\partial^2 u}{\partial y^2}\right) + \left(\frac{D_m}{m_H}m + \frac{\lambda_m}{m_H}\right)\left(\frac{\partial k_x}{\partial x} + \frac{\partial k_y}{\partial y}\right)\\ &+ \frac{\xi_m}{m_H}\left(\frac{\partial^3 k_x}{\partial x^3} + \frac{\partial^3 k_x}{\partial x \partial y^2} + \frac{\partial^3 k_y}{\partial x^2 \partial y} + \frac{\partial^3 k_y}{\partial y^3}\right),\end{aligned} \tag{S90}$$

where $M_x$, $M_y$, $m$, $k_x$, and $k_y$ are functions of $u$, see Eqs. (S87) and (S88). The force balance equation remains unchanged (except for the dislocation-related force, i.e. the $\mu_d$ term, which is set to zero in all numerical evaluations performed here).

### B. Mapping to previous work on active smectics without dislocations.

We are interested in mapping our theory without dislocations to that presented in Ref. [2]. We compare the linearized equations around the equilibrium state $m_0 = m_S = m_H$ and $\boldsymbol{k} = \hat{\boldsymbol{y}}$. Our linearized equation reads:

$$\frac{\partial \delta u}{\partial t} = D_m\frac{\partial^2 \delta u}{\partial y^2} - \frac{\xi_m}{m_H}\nabla^2\nabla^2\delta u - \frac{\lambda_m}{m_H}\frac{\partial^2 \delta u}{\partial x^2} + \frac{\xi_m}{m_H}\left(\frac{\partial^4 \delta u}{\partial x^2 \partial y^2} + \frac{\partial^4 \delta u}{\partial y^4}\right) + \delta v_y, \tag{S91}$$

where $\delta u$ and $\delta v_y$ are the perturbations around the equilibrium state.

In contrast, in the free energy framework presented in [1, 2], the linearized equation is

$$\frac{\partial \delta u}{\partial t} = \chi_v \left( \frac{\partial^2 \delta v_x}{\partial y^2} - \frac{\partial^2 \delta v_y}{\partial x \partial y} \right) + \Lambda_1 \frac{\partial^2 \delta u}{\partial y^2} - \Lambda_2 \nabla^2 \delta u + \chi \frac{\partial^2 \delta u}{\partial x \partial y} + \Gamma_u B \frac{\partial^2 \delta u}{\partial y^2} - \Gamma_u K \nabla^2 \nabla^2 \delta u + \delta v_y, \tag{S92}$$

where $B$ and $K$ are elastic constants for layer compression and layer bending deformations; $\Lambda_1$ and $\Lambda_2$ are active, achiral permeative terms; $\chi_v$ is a chiral velocity coupling coefficient; $\chi$ is an active chiral permeative term.

Comparing our formulation Eq. (S91) with the one of previous work (S92), we obtain the following mapping of parameters:

$$\chi_v = 0 \quad , \quad \chi = 0 \quad , \quad \Lambda_1 = \Lambda_2 = \frac{\lambda_m}{m_H}, \quad D_m = \Gamma_u B \quad , \quad \frac{\xi_m}{m_H} = \Gamma_u K. \tag{S93}$$

### C. Linear stability analysis

The uniform non-flowing steady state of the active smectics reads: $m = m_0$, $\boldsymbol{k} = \hat{\boldsymbol{y}}$, $\nabla u = (1 - m_0/m_H)\hat{\boldsymbol{y}}$, and $\boldsymbol{v} = \boldsymbol{0}$, where $m_0 = 1/a_0$ with $a_0$ being the initial layer thickness.

Next, we analyze the stability of the homogeneous steady state. The linearized perturbation equations read:

$$\frac{\partial \delta u}{\partial t} = D_m \nabla^2 \delta u + \frac{(m_0 D_m + \lambda_m)}{m_H} \left( \frac{\partial \delta k_x}{\partial x} + \frac{\partial \delta k_y}{\partial y} \right) + \frac{\xi_m}{m_H} \left( \frac{\partial^3 \delta k_x}{\partial x^3} + \frac{\partial^3 \delta k_x}{\partial x \partial y^2} + \frac{\partial^3 \delta k_y}{\partial x^2 \partial y} + \frac{\partial^3 \delta k_y}{\partial y^3} \right) + \frac{m_0}{m_H} \delta v_y, \tag{S94}$$

$$-\lambda \delta v_y + \eta \nabla^2 \delta v_y = \frac{\partial \delta P}{\partial y} + \frac{\partial \delta \mathrm{X}}{\partial y} - \frac{\partial \delta \mathrm{Y}}{\partial x} - \delta T_y, \tag{S95}$$

$$\nabla^2 \delta P = \frac{\partial^2 \delta \mathrm{X}}{\partial x^2} - \frac{\partial^2 \delta \mathrm{X}}{\partial y^2} + 2\frac{\partial^2 \delta \mathrm{Y}}{\partial x \partial y} + \frac{\partial \delta T_x}{\partial x} + \frac{\partial \delta T_y}{\partial y}. \tag{S96}$$

Since

$$\delta m = -m_H \frac{\partial \delta u}{\partial y} \quad , \quad \delta \boldsymbol{k} = -\frac{m_H}{m_0} \frac{\partial \delta u}{\partial x} \hat{\boldsymbol{x}} \quad \Rightarrow \quad \delta k_x = -\frac{m_H}{m_0} \frac{\partial \delta u}{\partial x} \quad , \quad \delta k_y = 0, \tag{S97}$$

$$\delta \mathrm{X} = \frac{B}{2m_H} \delta m - K \left( \frac{\partial^2 \delta k_x}{\partial x \partial y} + \frac{\partial^2 \delta k_y}{\partial y^2} \right) = -\frac{1}{2} B \frac{\partial \delta u}{\partial y} + K \frac{m_H}{m_0} \frac{\partial^3 \delta u}{\partial x^2 \partial y}, \tag{S98}$$

$$\delta \mathrm{Y} = -B \frac{m_0 - m_S}{m_H} \delta k_x + K \left( \frac{\partial^2 \delta k_x}{\partial x^2} + \frac{\partial^2 \delta k_y}{\partial x \partial y} \right) = B \frac{m_0 - m_S}{m_0} \frac{\partial \delta u}{\partial x} - K \frac{m_H}{m_0} \frac{\partial^3 \delta u}{\partial x^3}, \tag{S99}$$

$$\delta T_x = -\zeta_b \frac{\partial \delta k_x}{\partial y} - \chi \frac{\partial \delta m}{\partial x} = \left( \zeta_b \frac{m_H}{m_0} + \chi m_H \right) \frac{\partial^2 \delta u}{\partial x \partial y}, \tag{S100}$$

$$\delta T_y = -\zeta_s \left( \frac{\partial \delta k_x}{\partial x} + \frac{\partial \delta k_y}{\partial y} \right) - \zeta_b \frac{\partial \delta k_y}{\partial y} - \chi \frac{\partial \delta m}{\partial y} = \zeta_s \frac{m_H}{m_0} \frac{\partial^2 \delta u}{\partial x^2} + \chi m_H \frac{\partial^2 \delta u}{\partial y^2}, \tag{S101}$$

the perturbation equations can be re-expressed as:

$$\frac{\partial \delta u}{\partial t} = D_m \nabla^2 \delta u - \left( D_m + \frac{\lambda_m}{m_0} \right) \frac{\partial^2 \delta u}{\partial x^2} - \frac{\xi_m}{m_0} \left( \frac{\partial^4 \delta u}{\partial x^4} + \frac{\partial^4 \delta u}{\partial x^2 \partial y^2} \right) + \frac{m_0}{m_H} \delta v_y, \tag{S102}$$

$$-\lambda \delta v_y + \eta \nabla^2 \delta v_y = \frac{\partial \delta P}{\partial y} - \left( \zeta_s \frac{m_H}{m_0} + B \frac{m_0 - m_S}{m_0} \right) \frac{\partial^2 \delta u}{\partial x^2} - \left( \frac{1}{2} B + \chi m_H \right) \frac{\partial^2 \delta u}{\partial y^2} + K \frac{m_H}{m_0} \frac{\partial^4 \delta u}{\partial x^4} + K \frac{m_H}{m_0} \frac{\partial^4 \delta u}{\partial x^2 \partial y^2}, \tag{S103}$$

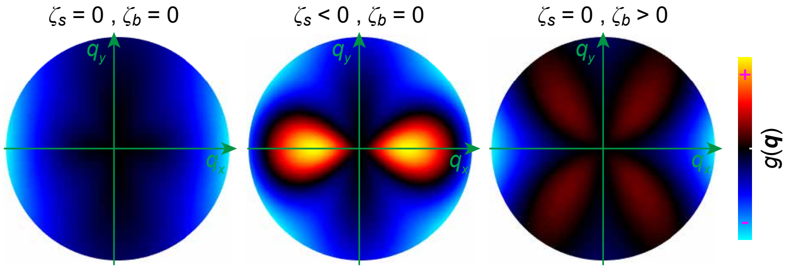


FIG. S6: Typical patterns of the mode growth rate $g(\boldsymbol{q})$ (see Eq. (S110)) in the Fourier space. (a) Passive case: $\zeta_s = \zeta_b = 0$. (b, c) Active case: (b) Role of $\zeta_s$, $\zeta_s < 0$ and $\zeta_b = 0$; (c) Role of $\zeta_b$: $\zeta_s = 0$ and $\zeta_b > 0$.

$$\nabla^2 \delta P = \Big[B\frac{3m_0 - 4m_S}{2m_0} + m_H\Big(\frac{\zeta_s+\zeta_b}{m_0} + \chi\Big)\Big]\frac{\partial^3 \delta u}{\partial x^2 \partial y} + \Big(\frac{1}{2}B + \chi m_H\Big)\frac{\partial^3 \delta u}{\partial y^3} - K\frac{m_H}{m_0}\frac{\partial^5 \delta u}{\partial x^4 \partial y} - K\frac{m_H}{m_0}\frac{\partial^5 \delta u}{\partial x^2 \partial y^3}. \tag{S104}$$

In the Fourier space, these perturbation equations read,

$$\frac{\partial \widetilde{\delta u}}{\partial t} = -D_m q^2 \widetilde{\delta u} + \Big(D_m + \frac{\lambda_m}{m_0}\Big) q_x^2 \widetilde{\delta u} - \frac{\xi_m}{m_0} q^2 q_x^2 \widetilde{\delta u} + \frac{m_0}{m_H}\widetilde{\delta v_y}, \tag{S105}$$

$$\widetilde{\delta v_y} = -\mathrm{i}\frac{q_y}{(\lambda+\eta q^2)}\widetilde{\delta P} - \frac{1}{(\lambda+\eta q^2)}\Big[\Big(\zeta_s\frac{m_H}{m_0} + B\frac{m_0 - m_S}{m_0}\Big)q_x^2 + \Big(\frac{1}{2}B + \chi m_H\Big)q_y^2 + K\frac{m_H}{m_0}q^2 q_x^2\Big]\widetilde{\delta u}, \tag{S106}$$

$$\widetilde{\delta P} = \mathrm{i}\left\{\left[B\frac{3m_0 - 4m_S}{2m_0} + m_H\left(\frac{\zeta_s+\zeta_b}{m_0} + \chi\right)\right]q_x^2 + \left(\frac{1}{2}B + \chi m_H\right)q_y^2 + K\frac{m_H}{m_0}q^2 q_x^2\right\}\frac{q_y}{q^2}\widetilde{\delta u}, \tag{S107}$$

where $\widetilde{(\cdot)}$ refers to the Fourier transform. Substituting Eq. (S107) into Eq. (S106), we obtain

$$\widetilde{\delta v_y} = \frac{q_x^2}{(\lambda+\eta q^2)}\left[-\left(\zeta_s\frac{m_H}{m_0} + B\frac{m_0 - m_S}{m_0}\right)\frac{q_x^2}{q^2} + \left(\zeta_b\frac{m_H}{m_0} - B\frac{m_S}{m_0}\right)\frac{q_y^2}{q^2} - K\frac{m_H}{m_0}q_x^2\right]\widetilde{\delta u}, \tag{S108}$$

Further substituting Eqs. (S108) into Eq. (S105), we get

$$\frac{\partial \widetilde{\delta u}}{\partial t} = g(\boldsymbol{q})\,\widetilde{\delta u}, \tag{S109}$$

where

$$\begin{aligned} g(\boldsymbol{q}) = & -D_m q^2 \sin^2\phi + \frac{\lambda_m}{m_0}q^2\cos^2\phi - \frac{\xi_m}{m_0}q^4\cos^2\phi \\ & + \frac{q^2\cos^2\phi}{(\lambda+\eta q^2)}\Big[-\Big(\zeta_s + B\frac{m_0 - m_S}{m_H}\Big)\cos^2\phi + \Big(\zeta_b - B\frac{m_S}{m_H}\Big)\sin^2\phi - Kq^2\cos^2\phi\Big], \end{aligned} \tag{S110}$$

is the growth rate of the perturbation $\delta u$, with $\phi = \arg(\boldsymbol{q})$ being the argument of the wavevector $\boldsymbol{q}$ here. The stability of the uniform non-flowing state requires:

$$g(\boldsymbol{q}) < 0 \qquad (\forall \boldsymbol{q}). \tag{S111}$$

Figure S6 shows the landscape of $g(\boldsymbol{q})$ for different active traction parameters.

*Small-scale stability.* – We first consider small-scale perturbations, i.e., $q \to +\infty$. The leading-order terms in $b(q)$ and $c(q)$ read:

$$g(\boldsymbol{q} \to \infty) \simeq -\frac{\xi_m}{m_0}q^4\cos^2\phi < 0. \tag{S112}$$

This suggests that the active smectics system is always stable at small scales. In particular, in the limiting of $\xi_m \to 0$,

$$g(\boldsymbol{q} \to \infty) \simeq \Big( - D_m \sin^2\phi + \frac{\lambda_m}{m_0}\cos^2\phi - \frac{K}{\eta}\cos^4\phi \Big) q^2 < 0. \tag{S113}$$

This indicates the active smectic system is stable at small scales when $\xi_m \to 0$.

*Large-scale stability.* – We next consider large-scale perturbations, i.e., $q \to 0$. In such a limiting case, we have the leading-order terms:

$$g(\boldsymbol{q} \to 0) \simeq \left\{ -D_m + \left[ D_m + \frac{\lambda_m}{m_0} + \frac{1}{\lambda}\left(\zeta_b - B\frac{m_S}{m_H}\right)\right]\cos^2\phi - \frac{1}{\lambda}\left(\zeta_s + \zeta_b + B\frac{m_0 - 2m_S}{m_H}\right)\cos^4\phi \right\} q^2. \tag{S114}$$

The stability condition reads:

$$-D_m + \left[ D_m + \frac{\lambda_m}{m_0} + \frac{1}{\lambda}\left(\zeta_b - B\frac{m_S}{m_H}\right)\right]\cos^2\phi - \frac{1}{\lambda}\left(\zeta_s + \zeta_b + B\frac{m_0 - 2m_S}{m_H}\right)\cos^4\phi < 0 \quad (\forall\phi), \tag{S115}$$

which results in the following necessary condition:

$$\zeta_s > \zeta_s^{\mathrm{cr}}. \tag{S116}$$

for the layer stability, where

$$\zeta_s^{\mathrm{cr}} = -B\frac{m_0 - m_S}{m_H} + \frac{\lambda_m}{m_0}\lambda. \tag{S117}$$

The latter expression corresponds to Eq. (S71) in the absence of dislocations ; indeed, $K$, $m_H$, $\xi_m$, $\lambda$ and $\eta$ are all positive; $\lambda_m = \tilde{\lambda}_m$ in the absence of dislocations, and we assume that $\tilde{\lambda}_m$ is negative based on the constraint on the passive case (see Eq. (S53), then $\lambda_m$ is the minimal term in the expression of the critical active stress of Eq. (S71).

*Buckling.* – Here, we consider the perturbations along the smectic layers, i.e., $\phi = 0$. In this case,

$$g(\phi = 0) = \frac{\lambda_m}{m_0}q^2 - \frac{\xi_m}{m_0}q^4 - \frac{q^2}{(\lambda + \eta q^2)}\Big(\zeta_s + B\frac{m_0 - m_S}{m_H} + Kq^2\Big). \tag{S118}$$

The stability condition $g < 0$ results in the same expression for the critical active splay traction as Eq. (S117), i.e. for $\zeta_s < \zeta_s^{\mathrm{cr}}$ the active smectic layers will undergo buckling instability.

The stability condition $g < 0$ also leads to a critical $m_0$:

$$m_0^{\mathrm{cr}} = \frac{-\zeta_s m_H + B m_S + \sqrt{(\zeta_s m_H - B m_S)^2 + 4B\lambda_m \lambda m_H}}{2B}, \tag{S119}$$

below which buckling instability occurs. In particular, in the passive limit $\zeta_s = 0$ and $\lambda_m = 0$, $m_0^{\mathrm{cr}} = m_H$, as expected.

By letting $\mathrm{d}g/\mathrm{d}q = 0$, we get the characteristic wavenumber, denoted $q_c$, which satisfies the following equation:

$$2\frac{\xi_m}{m_0}\eta^2 q_c^6 - \eta\Big(\frac{\lambda_m}{m_0}\eta - 4\frac{\xi_m}{m_0}\lambda - K\Big)q_c^4 - 2\lambda\Big(\frac{\lambda_m}{m_0}\eta - \frac{\xi_m}{m_0}\lambda - K\Big)q_c^2 - \lambda\left(\zeta_s^{\mathrm{cr}} - \zeta_s\right) = 0. \tag{S120}$$

In particular, in the following limiting cases, we have some simple analytical expressions of $q_c$:

- In the limit of $\lambda \to 0$, i.e., zero friction case,

$$g(q) = -\frac{\xi_m}{m_0}q^4 - \Big(\frac{K}{\eta} - \frac{\lambda_m}{m_0}\Big)q^2 + \frac{1}{\eta}\left(\zeta_s^{\mathrm{cr}} - \zeta_s\right), \tag{S121}$$

  and Eq. (S120) simplifies to $q_c = 0$.

- In the limit of $\eta \to 0$, i.e., zero viscosity case,

$$g(q) = -\Big(\frac{\xi_m}{m_0} + \frac{K}{\lambda}\Big)q^4 + \frac{1}{\lambda}\left(\zeta_s^{\mathrm{cr}} - \zeta_s\right)q^2, \tag{S122}$$

  and Eq. (S120) simplifies to,

$$q_c = \sqrt{\frac{m_0\left(\zeta_s^{\mathrm{cr}} - \zeta_s\right)}{2\left(Km_0 + \xi_m\lambda - \lambda_m\eta\right)}}. \tag{S123}$$

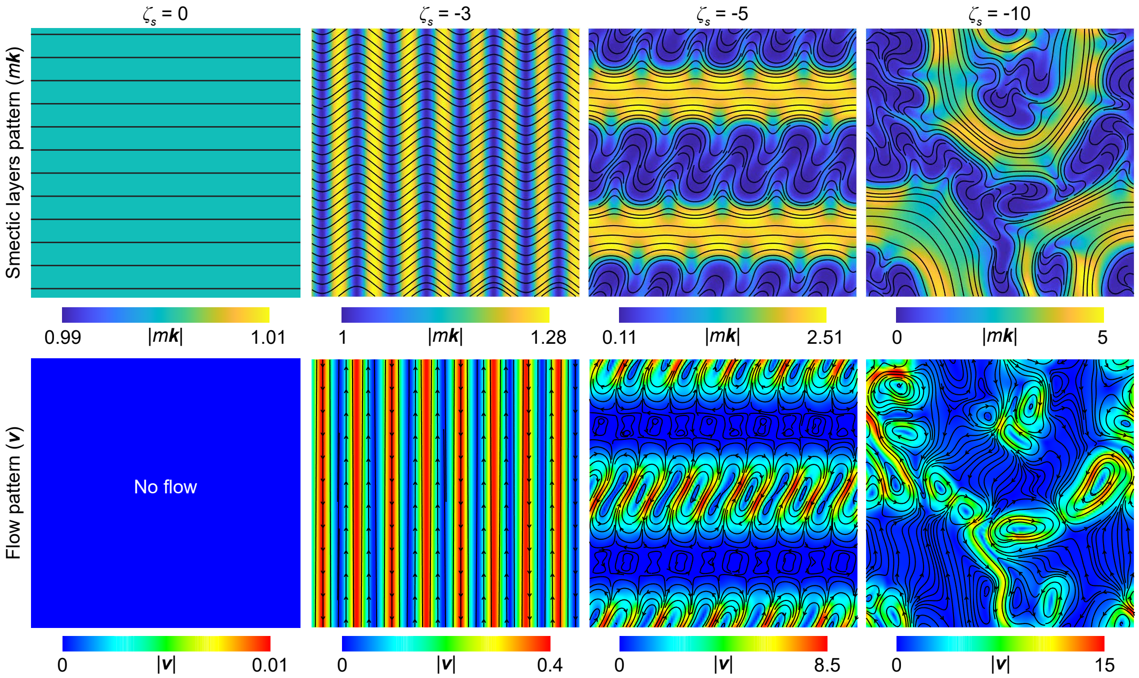


FIG. S7: Typical patterns of active smectic layers without dislocations driven by the active splay traction $\zeta_s$. (*Top*) Smectic layers pattern: the color code represents the magnitude $m = |m\boldsymbol{k}|$, and black lines denote smectic layers. (*Bottom*) Flow pattern: the color code represents the flow velocity magnitude $|\boldsymbol{v}|$, and the black lines with arrows denote streamlines. Parameters: $\lambda = 0.2$, $\eta = 1$, $\lambda_m = -1$, $D_m = 1$, $m_0 = m_H = m_S = 1$, $B = 10$, $K = 5$, $\zeta_b = 0$, and $\xi_m = 0.5$.

*Stability along the normal direction.–* We next consider the wave perturbations perpendicular to layers, i.e., $\phi = \pi/2$. In this case

$$g\Big(\phi = \frac{\pi}{2}\Big) = -D_m q^2. \tag{S124}$$

Thus, the active smectic layers are stable along the normal direction.

*Stability along the direction $\phi = \pi/4$.* – Our numerical calculations of $g(\boldsymbol{q})$ suggest that the active bend traction leads to instability along the direction $\phi = \pi/4$, see Fig. S6. In such a direction, we have

$$g\Big(\phi = \frac{\pi}{4}\Big) = -\frac{1}{2}D_m q^2 + \frac{1}{2}\frac{\lambda_m}{m_0}q^2 - \frac{1}{2}\frac{\xi_m}{m_0}q^4 + \frac{1}{4}\frac{q^2}{(\lambda+\eta q^2)}\Big(-\zeta_s + \zeta_b - B\frac{m_0}{m_H} - Kq^2\Big). \tag{S125}$$

The stability condition $g < 0$ results in a critical active bend traction,

$$\zeta_b^{\mathrm{cr}} = \zeta_s + B\frac{m_0}{m_H} + 2\lambda\Big(D_m - \frac{\lambda_m}{m_0}\Big), \tag{S126}$$

beyond which the homogeneous state will undergo instability. This is confirmed by our numerical simulations; see Fig. S7.


[1] F. Jülicher, J. Prost, and J. Toner, Physical Review E **106**, 054607 (2022).
[2] S. J. Kole, G. P. Alexander, S. Ramaswamy, and A. Maitra, Physical Review Letters **126**, 248001 (2021).
